# Supplementary material for: Exploring compactified HEIDI models at the LHC
Source: arXiv:1204.6264 source file (2012-04-27)
Supplement: Supplementary file 1 [file table_sm.tex]

\begin{tabular}{|lcl|l|lllllll|lll|}
\hline & & & & \multicolumn{7}{|c|}{\sc FeynRules} & \multicolumn{3}{|c|}{Stock}\\
\multicolumn{3}{|c|}{Process} & \multicolumn{1}{|c|}{$\sqrt{s}$}
 & \multicolumn{1}{|c}{CH} & \multicolumn{1}{c}{CH} & \multicolumn{1}{c}{MG}
 & \multicolumn{1}{c}{WO1} & \multicolumn{1}{c}{WO1} & \multicolumn{1}{c}{WO2}
 & \multicolumn{1}{c|}{WO2} & \multicolumn{1}{|c}{CH} & \multicolumn{1}{c}{MG}
 & \multicolumn{1}{c|}{WO2}\\
& & & \multicolumn{1}{c}{\scriptsize[GeV]} & \multicolumn{1}{|c}{F}
 & \multicolumn{1}{c}{U} & \multicolumn{1}{c}{U} & \multicolumn{1}{c}{F}
 & \multicolumn{1}{c}{U} & \multicolumn{1}{c}{F} & \multicolumn{1}{c|}{U}
 & \multicolumn{1}{|c}{U} & \multicolumn{1}{c}{U} & \multicolumn{1}{c|}{U}\\
\hline\hline
$\scriptstyle W^+\;W^+$ & $\scriptstyle\rightarrow$ & $\scriptstyle W^+\;W^+$ &
 $\scriptstyle 1277$ 
 & {\scriptsize 25.7} & {\scriptsize 25.7} & {\scriptsize 25.7} & {\scriptsize 25.7}
 & {\scriptsize 25.7} & {\scriptsize 25.7} & {\scriptsize 25.7} & {\scriptsize 25.7}
 & {\scriptsize 25.7} & {\scriptsize 25.7}
\\
$\scriptstyle g\;g$ & $\scriptstyle\rightarrow$ & $\scriptstyle g\;g$ &
 $\scriptstyle 200$ 
 & {\scriptsize 1.88e04} & {\scriptsize 1.88e04} & {\scriptsize 1.89e04}
 & {\scriptsize 1.88e04} & {\scriptsize 1.88e04} & {\scriptsize 1.88e04}
 & {\scriptsize 1.88e04} & {\scriptsize 1.88e04} & {\scriptsize 1.88e04}
 & {\scriptsize 1.88e04}
\\
$\scriptstyle Z\;Z$ & $\scriptstyle\rightarrow$ & $\scriptstyle W^+\;W^-$ &
 $\scriptstyle 1368$ 
 & {\scriptsize 26.2} & {\scriptsize 26.2} & {\scriptsize 26.2} & {\scriptsize 26.2}
 & {\scriptsize 26.2} & {\scriptsize 26.2} & {\scriptsize 26.2} & {\scriptsize 26.2}
 & {\scriptsize 26.2} & {\scriptsize 26.2}
\\
$\scriptstyle \gamma\;\gamma$ & $\scriptstyle\rightarrow$ & $\scriptstyle W^+\;W^-$ &
 $\scriptstyle 639$ 
 & {\scriptsize 16.3} & {\scriptsize 16.3} & {\scriptsize 16.3} & {\scriptsize 16.3}
 & {\scriptsize 16.3} & {\scriptsize 16.3} & {\scriptsize 16.3} & {\scriptsize 16.3}
 & {\scriptsize 16.3} & {\scriptsize 16.3}
\\
$\scriptstyle Z\;Z$ & $\scriptstyle\rightarrow$ & $\scriptstyle Z\;Z$ &
 $\scriptstyle 1459$ 
 & {\scriptsize 0.245} & {\scriptsize 0.245} & {\scriptsize 0.245} & {\scriptsize 0.245}
 & {\scriptsize 0.245} & {\scriptsize 0.245} & {\scriptsize 0.245} & {\scriptsize 0.245}
 & {\scriptsize 0.245} & {\scriptsize 0.245}
\\
$\scriptstyle \gamma\;Z$ & $\scriptstyle\rightarrow$ & $\scriptstyle W^+\;W^-$ &
 $\scriptstyle 1003$ 
 & {\scriptsize 19.3} & {\scriptsize 19.3} & {\scriptsize 19.3} & {\scriptsize 19.3}
 & {\scriptsize 19.3} & {\scriptsize 19.3} & {\scriptsize 19.3} & {\scriptsize 19.3}
 & {\scriptsize 19.3} & {\scriptsize 19.3}
\\\hline
$\scriptstyle s\;\bar{s}$ & $\scriptstyle\rightarrow$ & $\scriptstyle Z\;Z$ &
 $\scriptstyle 730$ 
 & {\scriptsize 0.0838} & {\scriptsize 0.0838} & {\scriptsize 0.0839}
 & {\scriptsize 0.0838} & {\scriptsize 0.0838} & {\scriptsize 0.0838}
 & {\scriptsize 0.0838} & {\scriptsize 0.0838} & {\scriptsize 0.0839}
 & {\scriptsize 0.0838}
\\
$\scriptstyle \mu^-\;\mu^+$ & $\scriptstyle\rightarrow$ & $\scriptstyle \gamma\;Z$ &
 $\scriptstyle 366$ 
 & {\scriptsize 1.46} & {\scriptsize 1.46} & {\scriptsize 1.46} & {\scriptsize 1.46}
 & {\scriptsize 1.46} & {\scriptsize 1.46} & {\scriptsize 1.46} & {\scriptsize 1.46}
 & {\scriptsize 1.46} & {\scriptsize 1.46}
\\
$\scriptstyle s\;\bar{s}$ & $\scriptstyle\rightarrow$ & $\scriptstyle \gamma\;\gamma$ &
 $\scriptstyle 200$ 
 & {\scriptsize 0.0272} & {\scriptsize 0.0272} & {\scriptsize 0.0272}
 & {\scriptsize 0.0272} & {\scriptsize 0.0272} & {\scriptsize 0.0272}
 & {\scriptsize 0.0272} & {\scriptsize 0.0272} & {\scriptsize 0.0272}
 & {\scriptsize 0.0272}
\\
$\scriptstyle u\;\bar{d}$ & $\scriptstyle\rightarrow$ & $\scriptstyle Z\;W^+$ &
 $\scriptstyle 684$ 
 & {\scriptsize 0.146} & {\scriptsize 0.146} & {\scriptsize 0.146} & {\scriptsize 0.146}
 & {\scriptsize 0.146} & {\scriptsize 0.146} & {\scriptsize 0.146} & {\scriptsize 0.146}
 & {\scriptsize 0.146} & {\scriptsize 0.146}
\\
$\scriptstyle c\;\bar{c}$ & $\scriptstyle\rightarrow$ & $\scriptstyle g\;g$ &
 $\scriptstyle 200$ 
 & {\scriptsize 462} & {\scriptsize 462} & {\scriptsize 462} & {\scriptsize 462}
 & {\scriptsize 462} & {\scriptsize 462} & {\scriptsize 462} & {\scriptsize 462}
 & {\scriptsize 462} & {\scriptsize 462}
\\
$\scriptstyle \nu_e\;e^+$ & $\scriptstyle\rightarrow$ & $\scriptstyle \gamma\;W^+$ &
 $\scriptstyle 319$ 
 & {\scriptsize 1.98} & {\scriptsize 1.98} & {\scriptsize 1.98} & {\scriptsize 1.98}
 & {\scriptsize 1.98} & {\scriptsize 1.98} & {\scriptsize 1.99} & {\scriptsize 1.98}
 & {\scriptsize 1.98} & {\scriptsize 1.98}
\\
$\scriptstyle d\;\bar{d}$ & $\scriptstyle\rightarrow$ & $\scriptstyle \gamma\;Z$ &
 $\scriptstyle 365$ 
 & {\scriptsize 0.0798} & {\scriptsize 0.0798} & {\scriptsize 0.0799}
 & {\scriptsize 0.0798} & {\scriptsize 0.0798} & {\scriptsize 0.0798}
 & {\scriptsize 0.0798} & {\scriptsize 0.0798} & {\scriptsize 0.0798}
 & {\scriptsize 0.0798}
\\
$\scriptstyle b\;\bar{b}$ & $\scriptstyle\rightarrow$ & $\scriptstyle Z\;Z$ &
 $\scriptstyle 767$ 
 & {\scriptsize 0.0760} & {\scriptsize 0.0760} & {\scriptsize 0.0758}
 & {\scriptsize 0.0760} & {\scriptsize 0.0760} & {\scriptsize 0.0760}
 & {\scriptsize 0.0760} & {\scriptsize 0.0760} & {\scriptsize 0.0758}
 & {\scriptsize 0.0760}
\\
$\scriptstyle c\;\bar{s}$ & $\scriptstyle\rightarrow$ & $\scriptstyle \gamma\;W^+$ &
 $\scriptstyle 325$ 
 & {\scriptsize 0.208} & {\scriptsize 0.208} & {\scriptsize 0.208} & {\scriptsize 0.207}
 & {\scriptsize 0.208} & {\scriptsize 0.208} & {\scriptsize 0.208} & {\scriptsize 0.208}
 & {\scriptsize 0.208} & {\scriptsize 0.208}
\\
$\scriptstyle \nu_\tau\;\bar{\nu}_\tau$ & $\scriptstyle\rightarrow$ &
 $\scriptstyle W^+\;W^-$ & $\scriptstyle 639$ 
 & {\scriptsize 1.06} & {\scriptsize 1.06} & {\scriptsize 1.06} & {\scriptsize 1.06}
 & {\scriptsize 1.06} & {\scriptsize 1.06} & {\scriptsize 1.06} & {\scriptsize 1.06}
 & {\scriptsize 1.06} & {\scriptsize 1.06}
\\\hline
$\scriptstyle \nu_\mu\;\bar{\nu}_\tau$ & $\scriptstyle\rightarrow$ &
 $\scriptstyle \mu^-\;\tau^+$ & $\scriptstyle 200$ 
 & {\scriptsize 16.5} & {\scriptsize 16.5} & {\scriptsize 16.5} & {\scriptsize 16.5}
 & {\scriptsize 16.5} & {\scriptsize 16.5} & {\scriptsize 16.5} & {\scriptsize 16.5}
 & {\scriptsize 16.5} & {\scriptsize 16.5}
\\
$\scriptstyle \nu_\mu\;\bar{\nu}_\mu$ & $\scriptstyle\rightarrow$ &
 $\scriptstyle \mu^-\;\mu^+$ & $\scriptstyle 200$ 
 & {\scriptsize 22.4} & {\scriptsize 22.4} & {\scriptsize 22.4} & {\scriptsize 22.4}
 & {\scriptsize 22.4} & {\scriptsize 22.4} & {\scriptsize 22.4} & {\scriptsize 22.4}
 & {\scriptsize 22.4} & {\scriptsize 22.4}
\\
$\scriptstyle t\;\bar{t}$ & $\scriptstyle\rightarrow$ & $\scriptstyle s\;\bar{s}$ &
 $\scriptstyle 1395$ 
 & {\scriptsize 1.14} & {\scriptsize 1.14} & {\scriptsize 1.14} & {\scriptsize 1.14}
 & {\scriptsize 1.14} & {\scriptsize 1.14} & {\scriptsize 1.14} & {\scriptsize 1.14}
 & {\scriptsize 1.14} & {\scriptsize 1.14}
\\
$\scriptstyle e^-\;e^+$ & $\scriptstyle\rightarrow$ & $\scriptstyle t\;\bar{t}$ &
 $\scriptstyle 1394$ 
 & {\scriptsize 0.0723} & {\scriptsize 0.0723} & {\scriptsize 0.0724}
 & {\scriptsize 0.0723} & {\scriptsize 0.0723} & {\scriptsize 0.0723}
 & {\scriptsize 0.0723} & {\scriptsize 0.0723} & {\scriptsize 0.0723}
 & {\scriptsize 0.0723}
\\
$\scriptstyle c\;c$ & $\scriptstyle\rightarrow$ & $\scriptstyle c\;c$ &
 $\scriptstyle 200$ 
 & {\scriptsize 3.41e03} & {\scriptsize 3.41e03} & {\scriptsize 3.42e03}
 & {\scriptsize 3.41e03} & {\scriptsize 3.41e03} & {\scriptsize 3.42e03}
 & {\scriptsize 3.41e03} & {\scriptsize 3.41e03} & {\scriptsize 3.41e03}
 & {\scriptsize 3.42e03}
\\
$\scriptstyle u\;\bar{u}$ & $\scriptstyle\rightarrow$ & $\scriptstyle s\;\bar{s}$ &
 $\scriptstyle 200$ 
 & {\scriptsize 80.3} & {\scriptsize 80.3} & {\scriptsize 80.2} & {\scriptsize 80.3}
 & {\scriptsize 80.3} & {\scriptsize 80.3} & {\scriptsize 80.3} & {\scriptsize 80.3}
 & {\scriptsize 80.3} & {\scriptsize 80.3}
\\
$\scriptstyle u\;\bar{u}$ & $\scriptstyle\rightarrow$ & $\scriptstyle d\;\bar{d}$ &
 $\scriptstyle 200$ 
 & {\scriptsize 68.1} & {\scriptsize 68.1} & {\scriptsize 68.0} & {\scriptsize 68.1}
 & {\scriptsize 68.1} & {\scriptsize 68.1} & {\scriptsize 68.1} & {\scriptsize 68.1}
 & {\scriptsize 68.1} & {\scriptsize 68.0}
\\
$\scriptstyle u\;\bar{t}$ & $\scriptstyle\rightarrow$ & $\scriptstyle d\;\bar{b}$ &
 $\scriptstyle 716$ 
 & {\scriptsize 5.49} & {\scriptsize 5.49} & {\scriptsize 5.49} & {\scriptsize 5.49}
 & {\scriptsize 5.49} & {\scriptsize 5.49} & {\scriptsize 5.49} & {\scriptsize 5.49}
 & {\scriptsize 5.50} & {\scriptsize 5.49}
\\
$\scriptstyle \nu_\tau\;\tau^+$ & $\scriptstyle\rightarrow$ & $\scriptstyle u\;\bar{s}$ &
 $\scriptstyle 200$ 
 & {\scriptsize 0.501} & {\scriptsize 0.501} & {\scriptsize 0.501} & {\scriptsize 0.501}
 & {\scriptsize 0.501} & {\scriptsize 0.501} & {\scriptsize 0.501} & {\scriptsize 0.501}
 & {\scriptsize 0.501} & {\scriptsize 0.501}
\\
$\scriptstyle \nu_\mu\;\mu^+$ & $\scriptstyle\rightarrow$ & $\scriptstyle c\;\bar{s}$ &
 $\scriptstyle 200$ 
 & {\scriptsize 9.33} & {\scriptsize 9.33} & {\scriptsize 9.32} & {\scriptsize 9.33}
 & {\scriptsize 9.33} & {\scriptsize 9.33} & {\scriptsize 9.33} & {\scriptsize 9.33}
 & {\scriptsize 9.33} & {\scriptsize 9.33}
\\\hline
$\scriptstyle Z\;Z$ & $\scriptstyle\rightarrow$ & $\scriptstyle H\;H$ &
 $\scriptstyle 1690$ 
 & {\scriptsize 0.250} & {\scriptsize 0.250} & {\scriptsize 0.250} & {\scriptsize 0.250}
 & {\scriptsize 0.250} & {\scriptsize 0.250} & {\scriptsize 0.250} & {\scriptsize 0.250}
 & {\scriptsize 0.250} & {\scriptsize 0.250}
\\
$\scriptstyle W^+\;W^-$ & $\scriptstyle\rightarrow$ & $\scriptstyle H\;H$ &
 $\scriptstyle 1599$ 
 & {\scriptsize 0.151} & {\scriptsize 0.151} & {\scriptsize 0.151} & {\scriptsize 0.151}
 & {\scriptsize 0.151} & {\scriptsize 0.151} & {\scriptsize 0.151} & {\scriptsize 0.151}
 & {\scriptsize 0.151} & {\scriptsize 0.151}
\\
$\scriptstyle t\;\bar{t}$ & $\scriptstyle\rightarrow$ & $\scriptstyle H\;H$ &
 $\scriptstyle 2354$ 
 & {\scriptsize 0.0593} & {\scriptsize 0.0593} & {\scriptsize 0.0593}
 & {\scriptsize 0.0593} & {\scriptsize 0.0593} & {\scriptsize 0.0593}
 & {\scriptsize 0.0593} & {\scriptsize 0.0593} & {\scriptsize 0.0593}
 & {\scriptsize 0.0593}
\\
$\scriptstyle \tau^-\;\tau^+$ & $\scriptstyle\rightarrow$ & $\scriptstyle H\;H$ &
 $\scriptstyle 974$ 
 & {\scriptsize 2.96e-06} & {\scriptsize 2.96e-06} & {\scriptsize 2.96e-06}
 & {\scriptsize 2.96e-06} & {\scriptsize 2.96e-06} & {\scriptsize 2.96e-06}
 & {\scriptsize 2.96e-06} & {\scriptsize 2.96e-06} & {\scriptsize 2.96e-06}
 & {\scriptsize 2.96e-06}
\\
$\scriptstyle b\;\bar{b}$ & $\scriptstyle\rightarrow$ & $\scriptstyle H\;H$ &
 $\scriptstyle 998$ 
 & {\scriptsize 6.33e-06} & {\scriptsize 6.33e-06} & {\scriptsize 6.33e-06}
 & {\scriptsize 6.33e-06} & {\scriptsize 6.33e-06} & {\scriptsize 6.33e-06}
 & {\scriptsize 6.33e-06} & {\scriptsize 6.33e-06} & {\scriptsize 6.33e-06}
 & {\scriptsize 6.33e-06}
\\\hline
\end{tabular}
